# Supplementary material for: Mapping the co-evolution of artificial intelligence, robotics, and the internet of things over 20 years (1998-2017)
Source: arXiv:2006.02366 source file (2020-06-03)
Supplement: Supplementary file 1 [file S1_Appendix.pdf]

***PloS One* Supporting Information Appendix S1**

Article title: Mapping the Co-Evolution of Artificial Intelligence, Robotics, and Internet of Things Over 20 Years (1998-2017)

Authors: Katy Börner[1a], Leonard E. Cross[a], Michael Gallant[a], Shutian Ma[a], Adam S. Martin[a], Elizabeth Record[a], Olga B. Scrivner[a], Haici Yang[a], and Jonathan M. Dilger[b]

[a] Cyberinfrastructure for Network Science Center, Luddy School of Informatics, Computing, and Engineering, Indiana University, Bloomington, IN 47408, USA

[b] Naval Surface Warfare Center Crane Division, Crane, IN 47522, USA
[1] Corresponding Author: Email: katy@indiana.edu

**This PDF file includes:**

Supplementary text
Figures S1 to S3
Tables S1 to S5

**Other supplementary materials for this manuscript include the following:**

Code was made available at https://github.com/cns-iu/AICoEvolution

## *Data*

Data used in this study comprises stakeholder needs and user study results, publication and funding data as well as keyword dictionaries and other data files needed for keyword extraction.

***Stakeholder Needs and User studies*** include the Qualtrics survey materials (6 demographic questions, 24 questions with 5 visualizations) results available at https://github.com/cns-iu/AICoEvolution. Participants fell into two age groups: 31-40 age group (2) and 51-60 age group (3). One participant was female and 4 were male. All five were native English speakers.

***Publication data*** was retrieved from the IUNI Web of Science (WoS) Data Enclave (Indiana University Network Science Institute, 2018) and Clarivate Web-of-Science Portal. There exist 66,036,893 publications for the period 2010-2017. Exactly 32,716 publications are extracted with 291 publications overlapping.

***Funding data*** was retrieved from the NSF Award Search Portal NSF portal - https://nsf.gov/awardsearch and downloaded in bulk from https://nsf.gov/awardsearch/download.jsp

### Dictionaries

Other datasets include a stopword list from the Stanford natural language processing (NLP) library (Pan, Yan, Wang, & Hua, 2015), extracted WoS keywords related to AI, robotics, and IoT, the UCSD Map of Science and Classification System (Börner et al., 2012) available at https://cns.iu.edu/2012-UCSDMap.html and the list of abbreviation used to describe funding agencies and organizations on WoS portal available at https://github.com/cns-iu/AICoEvolution.

### *Code*

Software used in this study includes term entity extraction algorithms to identify keywords in funding titles and descriptions; algorithms to compute term frequency bursts, and network layout algorithms and tools such as Gephi, Make-a-Viz, and OpenRefine.

### Term Extraction

MaxMatch algorithm (Wong & Chan, 1996) was used to extract keywords from publication and funding data. For more details see https://github.com/cns-iu/cjobs (Börner et al., 2018).

## *Methods*

***Burst Detection and Visualization.*** Kleinberg's (2002) burst detection algorithm is used to detect sudden increases in how often certain keywords are used in temporal data streams.

***Co-Author Networks***. The Sci2 Tool was used to extract a co-author network using the co-author column.

***Network Layout Algorithms.*** Gephi (Version 0.9.2) (Bastian, Heymann, & Jacomy, 2009) was used to compute data overlays with the following plugins:

- **ForceAtlas2** was used to layout the *Co-Author Network* figure.
- **GeoLayout** was used to create 1) the *Co-Author network overlaid on US map* with mercator basemap and the *Temporal Convergence* figure using latitude and longitude coordinates to display nodes.

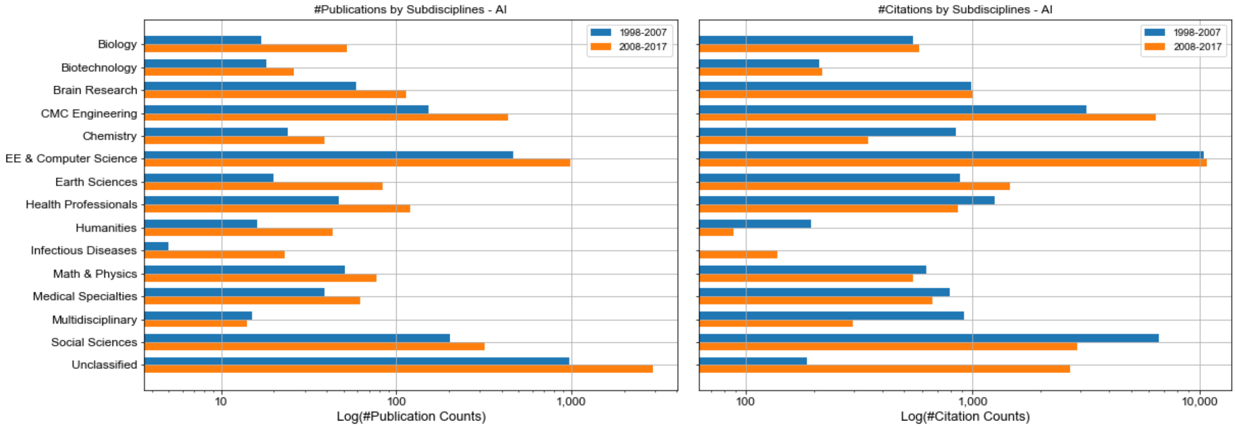


**S1 Fig.** Topical coverage of AI publications published in 1998-2007 and 2008-2017 in terms of number of papers (left) and number of citations (right). Abbreviations used: CMC – Chemical, Mechanical, and Civil; EE – Electrical Engineering).

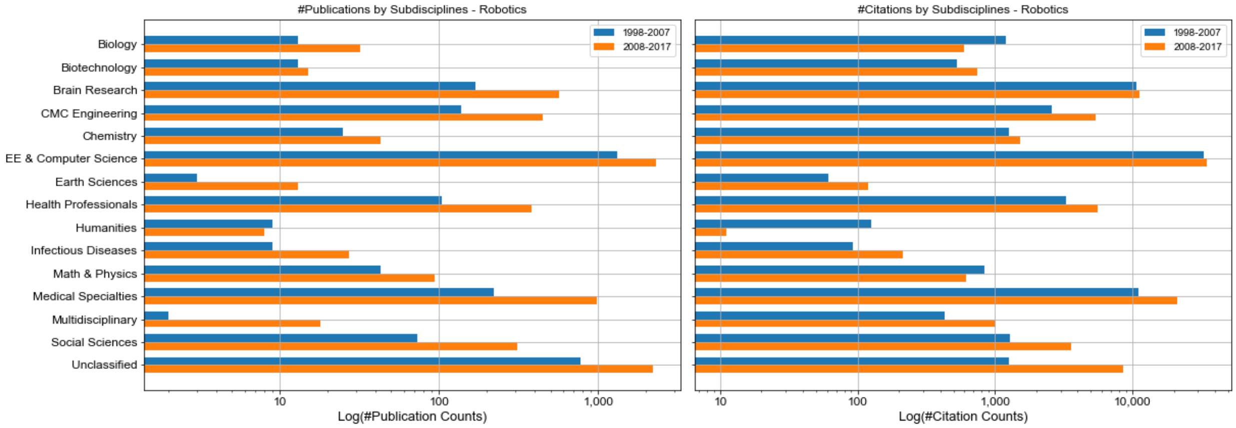


**S2 Fig.** Topical coverage of Robotics publications published in 1998-2007 and 2008-2017 in terms of number of papers (left) and number of citations (right).

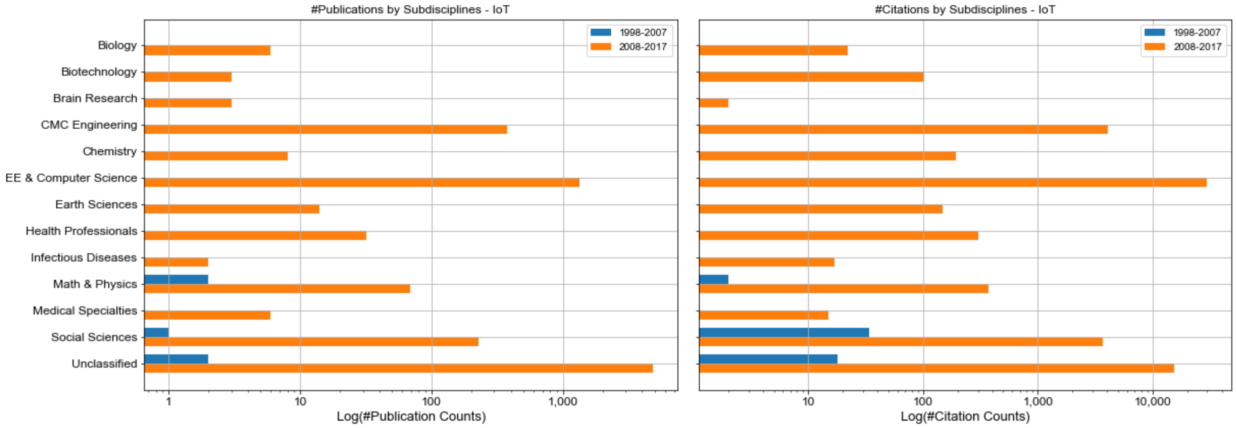


**S3 Fig.** Topical coverage of IoT publications published in 1998-2007 and 2008-2017 in terms of number of papers (left) and number of citations (right).

**Table S1**. Table Summary for S1 Fig - Topical coverage of AI publications published in 1998-2007 and 2008-2017 in terms of number of papers and number of citations. Unclassified labels and NULL labels were combined into Unclassified discipline.

| | 1998-2007 | | 2008-2017 | | | |
|---|---|---|---|---|---|---|
| **Disciplines** | **#Publications** | **#Citation** | **#Publications** | **#Citation** | **#Total Pubs** | **#Total Citations** |
| Biology | 17 | 549 | 52 | 584 | 69 | 1133 |
| Biotechnology | 18 | 211 | 26 | 218 | 44 | 429 |
| Brain Research | 59 | 990 | 114 | 1005 | 173 | 1995 |
| Chemical, Mechanical, & Civil Engineering | 152 | 3182 | 436 | 6432 | 588 | 9614 |
| Chemistry | 24 | 847 | 39 | 345 | 63 | 1192 |
| Earth Sciences | 20 | 876 | 84 | 1469 | 104 | 2345 |
| Electrical Engineering & Computer Science | 462 | 10480 | 982 | 10853 | 1444 | 21333 |
| Health Professionals | 47 | 1251 | 120 | 865 | 167 | 2116 |
| Humanities | 16 | 194 | 43 | 88 | 59 | 282 |
| Infectious Diseases | 5 | 58 | 23 | 138 | 28 | 196 |
| Math & Physics | 51 | 623 | 77 | 548 | 128 | 1171 |
| Medical Specialties | 39 | 795 | 62 | 668 | 101 | 1463 |
| Multidisciplinary | 15 | 913 | 14 | 296 | 29 | 1209 |
| Social Sciences | 203 | 6661 | 318 | 2883 | 521 | 9544 |
| Unclassified | 974 | 185 | 2922 | 2696 | 3896 | 2881 |
| Total | 2102 | 27815 | 5312 | 29088 | 7414 | 56903 |

**Table S2**. Table Summary for S2 Fig - Topical coverage of Robotics publications published in 1998-2007 and 2008-2017 in terms of number of papers and number of citations. Unclassified labels and NULL labels were combined into Unclassified discipline.

| | 1998-2007 | | 2008-2017 | | | |
|---|---|---|---|---|---|---|
| **Disciplines** | **#Publications** | **#Citations** | **#Publications** | **#Citations** | **#Total Pubs** | **#Total Citations** |
| Biology | 13 | 1206 | 32 | 594 | 45 | 1800 |
| Biotechnology | 13 | 527 | 15 | 746 | 28 | 1273 |
| Brain Research | 169 | 10772 | 569 | 11188 | 738 | 21960 |
| Chemical, Mechanical, & Civil Engineering | 138 | 2605 | 445 | 5376 | 583 | 7981 |
| Chemistry | 25 | 1272 | 43 | 1531 | 68 | 2803 |
| Earth Sciences | 3 | 61 | 13 | 120 | 16 | 181 |

| | | | | | | |
|---|---|---|---|---|---|---|
| Electrical Engineering & Computer Science | 1310 | 33083 | 2311 | 35043 | 3621 | 68126 |
| Health Professionals | 104 | 3281 | 381 | 5563 | 485 | 8844 |
| Humanities | 9 | 125 | 8 | 11 | 17 | 136 |
| Infectious Diseases | 9 | 93 | 27 | 215 | 36 | 308 |
| Math & Physics | 43 | 841 | 94 | 614 | 137 | 1455 |
| Medical Specialties | 221 | 11028 | 981 | 21181 | 1202 | 32209 |
| Multidisciplinary | 2 | 431 | 18 | 1016 | 20 | 1447 |
| Social Sciences | 73 | 1281 | 308 | 3581 | 381 | 4862 |
| Unclassified | 1689 | 1262 | 4865 | 8518 | 6554 | 9780 |
| Total | 3821 | 67868 | 10110 | 95297 | 13931 | 163165 |

**Table S3**. Table Summary for S3 Fig - Topical coverage of IoT publications published in 1998-2007 and 2008-2017 in terms of number of papers and number of citations. Unclassified labels and NULL labels were combined into Unclassified discipline.

| | 1998-2007 | | 2008-2017 | | | |
|---|---|---|---|---|---|---|
| Disciplines | #Publications | #Citations | #Publications | #Citations | #Total Pubs | #Total Citations |
| Biology | 0 | 0 | 6 | 22 | 6 | 22 |
| Biotechnology | 0 | 0 | 3 | 103 | 3 | 103 |
| Brain Research | 0 | 0 | 3 | 2 | 3 | 2 |
| Chemical, Mechanical, & Civil Engineering | 0 | 0 | 377 | 4110 | 377 | 4110 |
| Chemistry | 0 | 0 | 8 | 194 | 8 | 194 |
| Earth Sciences | 0 | 0 | 14 | 147 | 14 | 147 |
| Electrical Engineering & Computer Science | 0 | 0 | 1338 | 29997 | 1338 | 29997 |
| Health Professionals | 0 | 0 | 32 | 302 | 32 | 302 |
| Infectious Diseases | 0 | 0 | 2 | 17 | 2 | 17 |
| Math & Physics | 2 | 2 | 69 | 374 | 71 | 376 |

| | | | | | | |
|---|---|---|---|---|---|---|
| Medical Specialties | 0 | 0 | 6 | 15 | 6 | 15 |
| Social Sciences | 1 | 34 | 226 | 3665 | 227 | 3699 |
| Unclassified | 4 | 18 | 9280 | 15469 | 9284 | 15487 |
| Total | 7 | 54 | 11364 | 54417 | 11371 | 54471 |

**Table S4.** Top-5 research articles by #Citations.

| Title | Year | #Citation |
|---|---|---|
| **AI** | | |
| Artificial neural networks (the multilayer perceptron) - A review of … | 1998 | 681 |
| Psychological aspects of natural language use: Our words, our … | 2003 | 735 |
| Advances in Diagnostic Techniques for Induction Machines | 2008 | 559 |
| ViBe: A Universal Background Subtraction Algorithm for Video Sequ... | 2011 | 702 |
| A review on the prediction of building energy consumption | 2012 | 440 |
| **Robotics** | | |
| Vision for mobile robot navigation: A survey | 2002 | 609 |
| An inexpensive, automation-friendly protocol for recovering high-qual… | 2006 | 705 |
| Effects of robot-assisted therapy on upper limb recovery after stroke... | 2008 | 682 |
| A survey of robot learning from demonstration | 2009 | 721 |
| A review of shape memory alloy research, applications and opportunities | 2014 | 700 |
| **IoT** | | |
| The Internet of Things: A survey | 2010 | 3,859 |
| Internet of Things (IoT): A vision, architectural elements, and future… | 2013 | 2,344 |
| Recommender systems survey | 2013 | 693 |
| Internet of Things in Industries: A Survey | 2014 | 733 |
| Internet of Things: A Survey on Enabling Technologies, Protocols... | 2015 | 902 |

*Note. Data Citation (top 5 publications sorted by Citation) is available in data section: https://github.com/cns-iu/AICoEvolution*

**Table S5.** Top 10 Bursts for each domain in Publications and NSF Awards

| Publications | Burst Strength | NSF Awards | Burst Strength |
|---|---|---|---|
| **AI** | | | |
| Learning (Artificial intelligence) | 39.29 | Machine learning | 13.04 |
| Machine learning | 26.41 | Education | 9.96 |
| Neural networks | 25.61 | Making | 9.20 |
| Distributed artificial intelligence | 20.47 | Big data | 8.97 |
| Deep learning | 18.49 | Building | 8.06 |
| Expert systems | 17.99 | Web | 7.85 |
| Big data | 16.17 | Interaction | 7.29 |
| Genetic algorithms | 11.12 | Society | 7.06 |
| Feature extraction | 10.58 | Deep learning | 7.05 |
| Internet of things | 9.35 | Data science | 7.01 |
| **Robotics** | | | |

| | | | |
|---|---|---|---|
| Soft robotics | 58.15 | Law | 31.55 |
| Cloud robotics | 23.38 | Recovery | 27.84 |
| Educational robotics | 19.49 | Impacts | 21.00 |
| Control technology | 15.33 | STEM | 19.91 |
| Social robotics | 14.29 | Algebraic geometry | 17.24 |
| 3d printing | 14.18 | School | 14.35 |
| Teleoperation | 13.98 | College | 13.86 |
| Marine robotics | 13.05 | Soft robotics | 13.70 |
| Welding | 12.96 | Machine learning | 13.56 |
| Laparoscopy | 12.87 | Biology | 12.60 |
| **IoT** | | | |
| RFID | 62.16 | Vehicles | 4.26 |
| The internet of things | 33.63 | Monitor | 4.16 |
| Radio frequency identification | 15.07 | Computation | 4.15 |
| 6Lowpan | 13.20 | Runtime | 3.47 |
| EPC | 13.18 | Integrated circuits | 3.47 |
| Future internet | 12.91 | Experiments | 3.32 |
| Fog computing | 12.06 | Robust | 3.30 |
| Edge computing | 10.38 | Community | 3.27 |
| Lora | 10.13 | Social | 3.01 |
| Lorawan | 10.01 | Vehicle | 2.98 |

## References


Bastian, M., Heymann, S., & Jacomy, M. (2009). Gephi: an open source software for exploring and manipulating networks. In E. Adar, M. Hurst, T. Finin, N. Glance, N. Nicolov, & B. Tseng (Eds.), *Proceedings of the Third International Conference on Weblogs and Social Media* (pp. 361–362). Menlo Park, California: The AAAI Press. Retrieved from https://gephi.org/users/publications/

Börner, K., Klavans, R., Patek, M., Zoss, A. M., Biberstine, J. R., Light, R. P., … Boyack, K. W. (2012). Design and update of a classification system: The UCSD map of science. *PLoS ONE*, *7*(7), e39464. https://doi.org/10.1371/journal.pone.0039464

Börner, K., Scrivner, O., Gallant, M., Ma, S., Liu, X., Chewning, K., … Evans, J. A. (2018). Skill discrepancies between research, education, and jobs reveal the critical need to supply soft skills for the data economy. *Proceedings of the National Academy of Sciences of the United States of America*, *115*(50), 12630–12637. https://doi.org/10.1073/pnas.1804247115

Indiana University Network Science Institute. (2018). Web of Science (WoS). Retrieved July 13, 2018, from http://iuni.iu.edu/resources/web-of-science

Kleinberg, J. (2002). Bursty and hierarchical structure in streams. In D. Hand, D. A. Keim, & R. NG (Eds.), *Proceedings of the Eighth ACM SIGKDD International Conference on Knowledge Discovery and Data Mining - KDD '02* (pp. 91–101). New York, New York, USA: ACM Press. https://doi.org/10.1145/775047.775061

Pan, X., Yan, E., Wang, Q., & Hua, W. (2015). Assessing the impact of software on science: A

bootstrapped learning of software entities in full-text papers. *Journal of Informetrics*, *9*(4), 860–871. https://doi.org/10.1016/J.JOI.2015.07.012

Sci2 Team. (2009). Science of Science (Sci2) Tool. Indiana University and SciTech Strategies. Retrieved from https://sci2.cns.iu.edu

Wong, P.-K., & Chan, C. (1996). Chinese word segmentation based on maximum matching and word binding force. *Proceedings of the 16th Conference on Computational Linguistics*, *1*, 200–203. Retrieved from http://citeseerx.ist.psu.edu/viewdoc/download?doi=10.1.1.14.3112&rep=rep1&type=pdf
